# Supplementary material for: Planet Hunters TESS IV: A massive, compact hierarchical triple star system TIC 470710327
Source: arXiv:2202.06964 source file (2022-02-14)
Supplement: Supplementary file 1 [file Appendix_Soetkin.tex]

\begin{table*}
%\begin{adjustwidth}{-.5in}{-.5in}

    \centering
 % \begin{threeparttable}
    \caption{Photometric observations of TIC~470710327. Data obtained from VizieR (\url{http://vizier.unistra.fr/vizier/sed/}).}
     \begin{tabular}{llcll}
        \hline \hline
        Passband & Effective wavelength [\AA]& Flux [erg s$^{-1}$cm$^{-2}$\AA$^{-1}$]& Magnitude &Ref.\\
        \hline
Johnson:U&3971.00 & 6.52e-13 $\pm$ 3.26e-14 &9.38& a\\
HIP:BT& 4203.01 & 6.40e-13 $\pm$ 1.19e-14 & 9.40&b  \\
HIP:BT& 4203.01 & 6.65e-13 $\pm$ 1.53e-14  & 9.36 &c  \\
Johnson:B &4442.03& 6.17e-13 $\pm$ 1.37e-14 &9.44 & d \\
Johnson:B &4442.03& 6.47e-13 $\pm$ 1.82e-14 &9.39 & e \\
SDSS:g' & 4819.97 &7.88e-13 $\pm$ 7.62e-16 &9.17& f\\
HIP:VT &5318.96& 5.30e-13 $\pm$ 9.54e-15 &9.60& b \\
HIP:VT &5318.96& 5.51e-13 $\pm$ 1.27e-14 &9.56& c \\
Johnson:V &5537.05& 5.48e-13 $\pm$ 5.28e-14 &9.57 & d \\
Johnson:V &5537.05& 4.73e-13 $\pm$ 9.78e-15& 9.73 & f \\
SDSS:r' &  6246.98 &4.70e-13 $\pm$ 1.54e-14 &9.73& f\\
Gaia:G & 6729.95&3.08e-13 $\pm$ 4.63e-15 & 10.19& h \\
SDSS:i' & 7634.91 & 3.17e-13 $\pm$ 7.19e-16 & 10.16& f\\
2MASS:J &12390.1&9.94e-14 $\pm$ 1.76e-15 &11.42 & i \\
Johnson:J &12500.21&9.96e-14 $\pm$ 1.92e-15 &11.42& j \\
Johnson:H &16300.16&4.08e-14 $\pm$ 1.02e-15 &12.39& j \\
2MASS:H &16494.77 &4.02e-14 $\pm$ 1.10e-15 &12.40&i \\
2MASS:Ks& 21637.85&1.52e-14 $\pm$ 2.56e-16 &13.46&i \\
Johnson:K &21900.25&1.46e-14 $\pm$ 1.25e-16 &13.50& j \\
WISE:W1&33500.11&2.99e-15 $\pm$ 5.34e-17 &15.23 & k \\
Johnson:L &34000.10 & 2.72e-15 $\pm$ 5.19e-17 &15.33&c\\
WISE:W2 &46000.19&8.56e-16 $\pm$ 1.56e-17 &16.58& k \\
Johnson:M &50299.90 & 6.64e-16 $\pm$ 1.18e-17&16.86&c\\
WISE:W3 &115598.23&2.24e-17 $\pm$ 6.73e-19 &20.54& k \\
WISE:W4 &220906.68&2.98e-18 $\pm$ 3.93e-19 &22.73& k \\
        \hline
     \end{tabular}
         \flushleft
    \begin{tablenotes}
      \small
      \item \textbf{Notes.} Data from: $^{\text{(a)}}$ \cite{Reed_2003}; $^{\text{(b)}}$ \cite{Fabricius_2002}; $^{\text{(c)}}$ \cite{Bourges_2017}; $^{\text{(d)}}$ \cite{Ammons_2006}; $^{\text{(e)}}$ \cite{Lasker_2006}; $^{\text{(f)}}$ \cite{Henden_2016}; $^{\text{(g)}}$ \cite{Droege_2007}; $^{\text{(h)}}$ \cite{Altmann_2017}; $^{\text{(i)}}$ \cite{Zacharias_2012}; $^{\text{(j)}}$ \cite{Cutri_2003}; $^{\text{(k)}}$ \cite{Cutri_2013}
    \end{tablenotes}
    \label{table_data_vizier}
%  \end{threeparttable}
%\end{adjustwidth}
\end{table*}
